# Supplementary material for: Quadratic to linear magnetoresistance tuning in TmB4
Source: arXiv:1901.02165 source file (2019-01-08)
Supplement: Supplementary file 1 [file supplemental.pdf]

# Supplemental Info: Quadratic to linear magnetoresistance tuning in $TmB_4$

Sreemanta Mitra,[1,*] Jeremy Goh Swee Kang,[1] John Shin,[2] Jin Quan Ng,[1] Sai Swaroop Sunku,[1,†] Tai Kong,[3,‡] Paul C. Canfield,[3] B. Sriram Shastry,[2] Pinaki Sengupta,[1] and Christos Panagopoulos[1,§]

[1]*Division of Physics and Applied Physics, School of Physical and Mathematical Sciences, Nanyang Technological University, 21, Nanyang Link 637371, Singapore.*

[2]*Department of Physics, University of California, Santa Cruz, California 95064, USA.*

[3]*Ames Laboratory, U.S. DOE and Department of Physics and Astronomy, Iowa State University, Ames, Iowa, 50011, USA.*

## I. $T$-LIMIT CALCULATION

The applicability of the theory of quantum linear magnetoresistance (*LMR*)[1–4] requires the following temperature ($T$) condition to be satisfied to ensure that $T$ is smaller than the Landau level spacing,

$$T_{\text{limit}} < \frac{eB\hbar}{m^* c k_B}\,, \tag{1}$$

where $m^*$ is the effective mass, $e$ is the electronic charge, $B$ is the applied magnetic field, $c$ is the speed of light in free space and $k_B$ is the Boltzmann constant. The right hand side of the inequality should have dimension of temperature.

$$\left[\frac{eB\hbar}{m^* c k_B}\right] = \frac{(\text{cm}^{3/2}\,\text{g}^{1/2}\,\text{s}^{-1}) \times (\text{g}^{1/2}\,\text{cm}^{-1/2}\,\text{s}^{-1}) \times (\text{g}\,\text{cm}^2\,\text{s}^{-1})}{(\text{g}) \times (\text{cm}\,\text{s}^{-1}) \times (\text{g}\,\text{cm}^2\,\text{s}^{-2}\,\text{K}^{-1})}$$

$$= \text{K}$$

Since our measurements on $TmB_4$ were performed for $B \leq 13\,\text{kOe}$, we take $B = 10\,\text{kOe}$ to calculate the upper bound of $T$. A reasonable approximation of the effective mass of the carriers of the pocket is $\sim 0.1 m_0$ ($m_0$ is electronic rest mass), which is calculated theoretically for $TmB_4$[5] and experimentally observed in the iso-structural $YB_4$[6]. Substituting to eq.1 we find,

$$T_{\text{limit}} < \frac{eB\hbar}{m^* c\, k_B}$$

$$= \frac{(4.8 \times 10^{-10}) \times (10^4) \times (1.0546 \times 10^{-27})}{(0.1 \times 9.1 \times 10^{-28}) \times (3 \times 10^{10}) \times (1.38 \times 10^{-16})}$$

$$= 13.4\,\text{K}$$

This is consistent with our previous experimental observation[7], where a quadratic growth is seen for higher $T$.

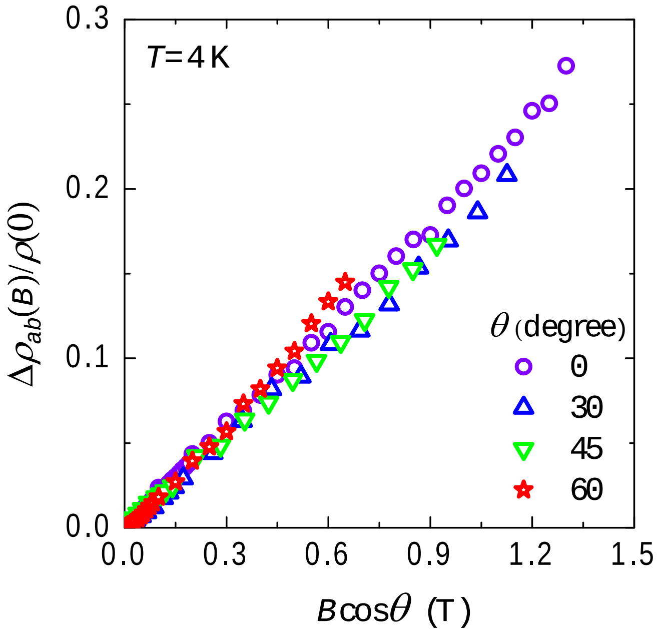


FIG. S1. The variation of $MR$ with $B\cos\theta$ for different direction of B, measured at $T = 4\,\mathrm{K}$

## II. ESTIMATION OF $N_i$

Since our crystals are grown in Al flux, a natural source of impurity will be Al[8]. Considering that the residual resistivity arises solely due to the impurity scattering, we estimate our crystal's impurity density ($N_i^{\mathrm{our}}$) by comparing its residual resistivity value ($\rho_0^{\mathrm{our}} = 12.9\,\Omega\,\mathrm{m}$) with that of a similarly prepared crystal ($\rho_0^{\mathrm{ref}} = 119\,\Omega\,\mathrm{m}$)[8], with known impurity density ($N_i^{\mathrm{ref}} \sim 1.08$ wt.%)[8]. Hence,

$$\frac{N_i^{\mathrm{our}}}{N_i^{\mathrm{ref}}} = \frac{\rho_0^{\mathrm{our}}}{\rho_0^{\mathrm{ref}}} \approx 0.1\,, \quad N_i^{\mathrm{our}} = 0.108\ \mathrm{wt.\%} \tag{2}$$

From the mass of our $TmB_4$ sample (0.35 mg), the above calculation suggests that it has 0.35 µg of Al impurity. This is equivalent to $1.29 \times 10^{-8}$ mol of Al. Normalizing with Avogadro's number, we estimate that the Al impurity density is of the order of $10^{21}\ \mathrm{m}^{-3}$.

---

* Current address: Department of Physics, Indian Institute of Science, Bangalore 560012, India. ; sreemanta85@gmail.com

† Present address: Department of Physics, Columbia University, New York, 10027, USA.

‡ Present address: Department of Chemistry, Princeton University, New Jersey, 08544, USA.

§ christos@ntu.edu.sg

[1] A. A. Abrikosov, Sov. Phys. JETP **29**, 746 (1969).

[2] A. A. Abrikosov, Phys. Rev. B **58**, 2788 (1998).

[3] A. A. Abrikosov, Phys. Rev. B **60**, 4231 (1999).

[4] A. A. Abrikosov, Europhys. Lett. **49**, 789 (2000).

[5] J. Shin, Z. Schlesinger, and B. S. Shastry, Phys. Rev. B **95**, 205140(9pp) (2017).

[6] T. Tanaka and Y. Ishizawa, J. Phys. C. **18**, 4933 (1985).

[7] S. S. Sunku, T. Kong, T. Ito, P. C. Canfield, B. S. Shastry, P. Sengupta, and C. Panagopoulos, Phys. Rev. B **93**, 174408(5pp) (2016).

[8] S. Okada, K. Kudou, Y. Yu, and T. Lundström, Jpn. J. Appl. Phys **33**, 2663 (1994).
